# Supplementary material for: Proca Stars with Dark Photons from Spontaneous Symmetry Breaking of the Scalar Field Dark Matter
Source: arXiv:2305.05674 source file (2023-05-09)
Supplement: Supplementary file 1 [file appendix1.tex]

\section{Appendix} \label{sec:appendix}
